# Supplementary material for: Neutral polymer conformations with attractive bridging crowder interactions: role of crowder size
Source: arXiv:2410.04113 ancillary file (2024-10-05)
Supplement: Supplementary file 1 [file Supp.pdf]

## Supporting Information

### **Neutral polymer conformations with attractive bridging crowder interactions: role of crowder size**

Hitesh Garg<sup>1, 2, a)</sup> and Satyavani Vemparala<sup>1, 2, b)</sup>

<sup>1)</sup>*The Institute of Mathematical Sciences, C.I.T. Campus, Taramani,  
Chennai 600113, India*

<sup>2)</sup>*Homi Bhabha National Institute, Training School Complex, Anushakti Nagar,  
Mumbai 400094, India*

(Dated: 5 October 2024)

---

<sup>a)</sup>Electronic mail: [hiteshgarg@imsc.res.in](mailto:hiteshgarg@imsc.res.in)

<sup>b)</sup>Electronic mail: [vani@imsc.res.in](mailto:vani@imsc.res.in)

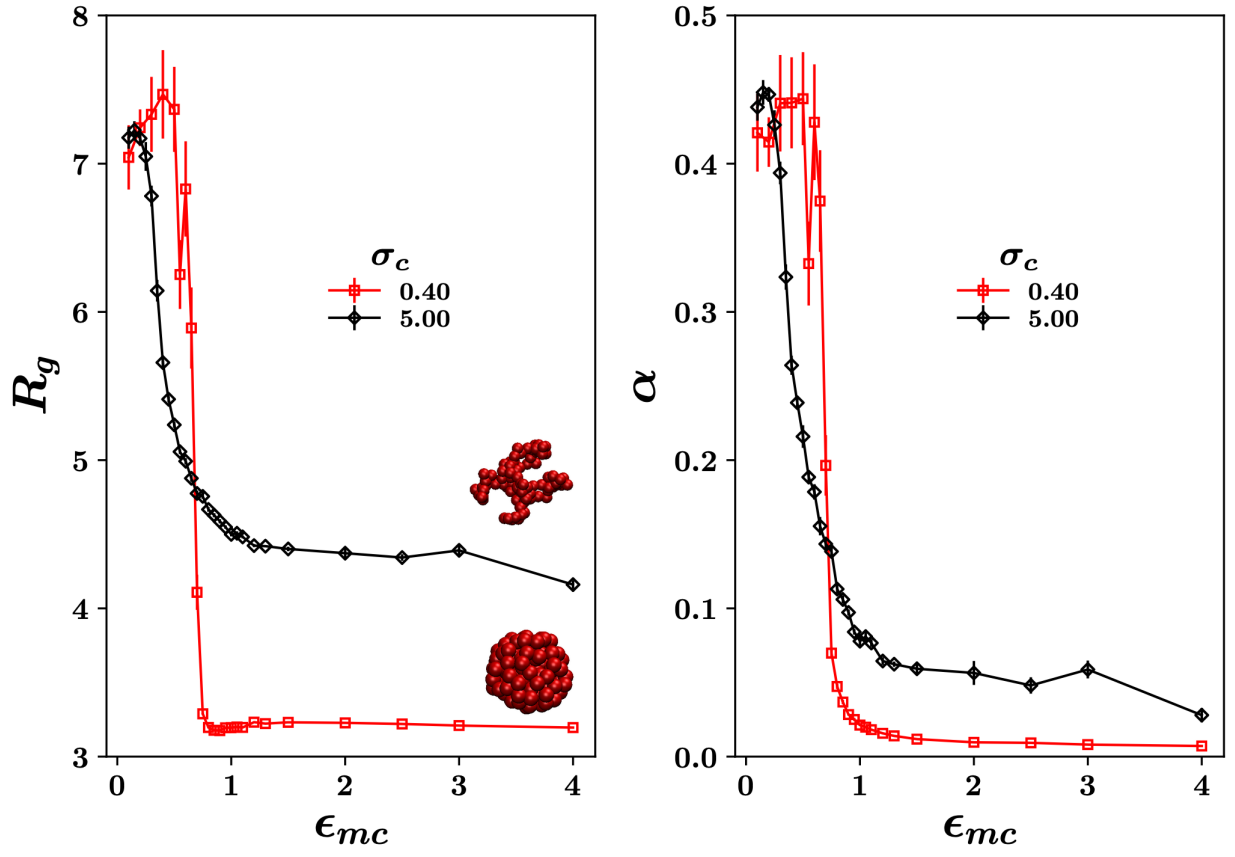

FIG. S1. The variation of the (a) radius of gyration,  $R_g$  and (b) asphericity  $\alpha$  with  $\epsilon_{mc}$  for smallest and largest crowder sizes  $\sigma_c = 0.4, 5.0$  considered in the study. The typical configurations of the polymer (without crowders) are also shown.

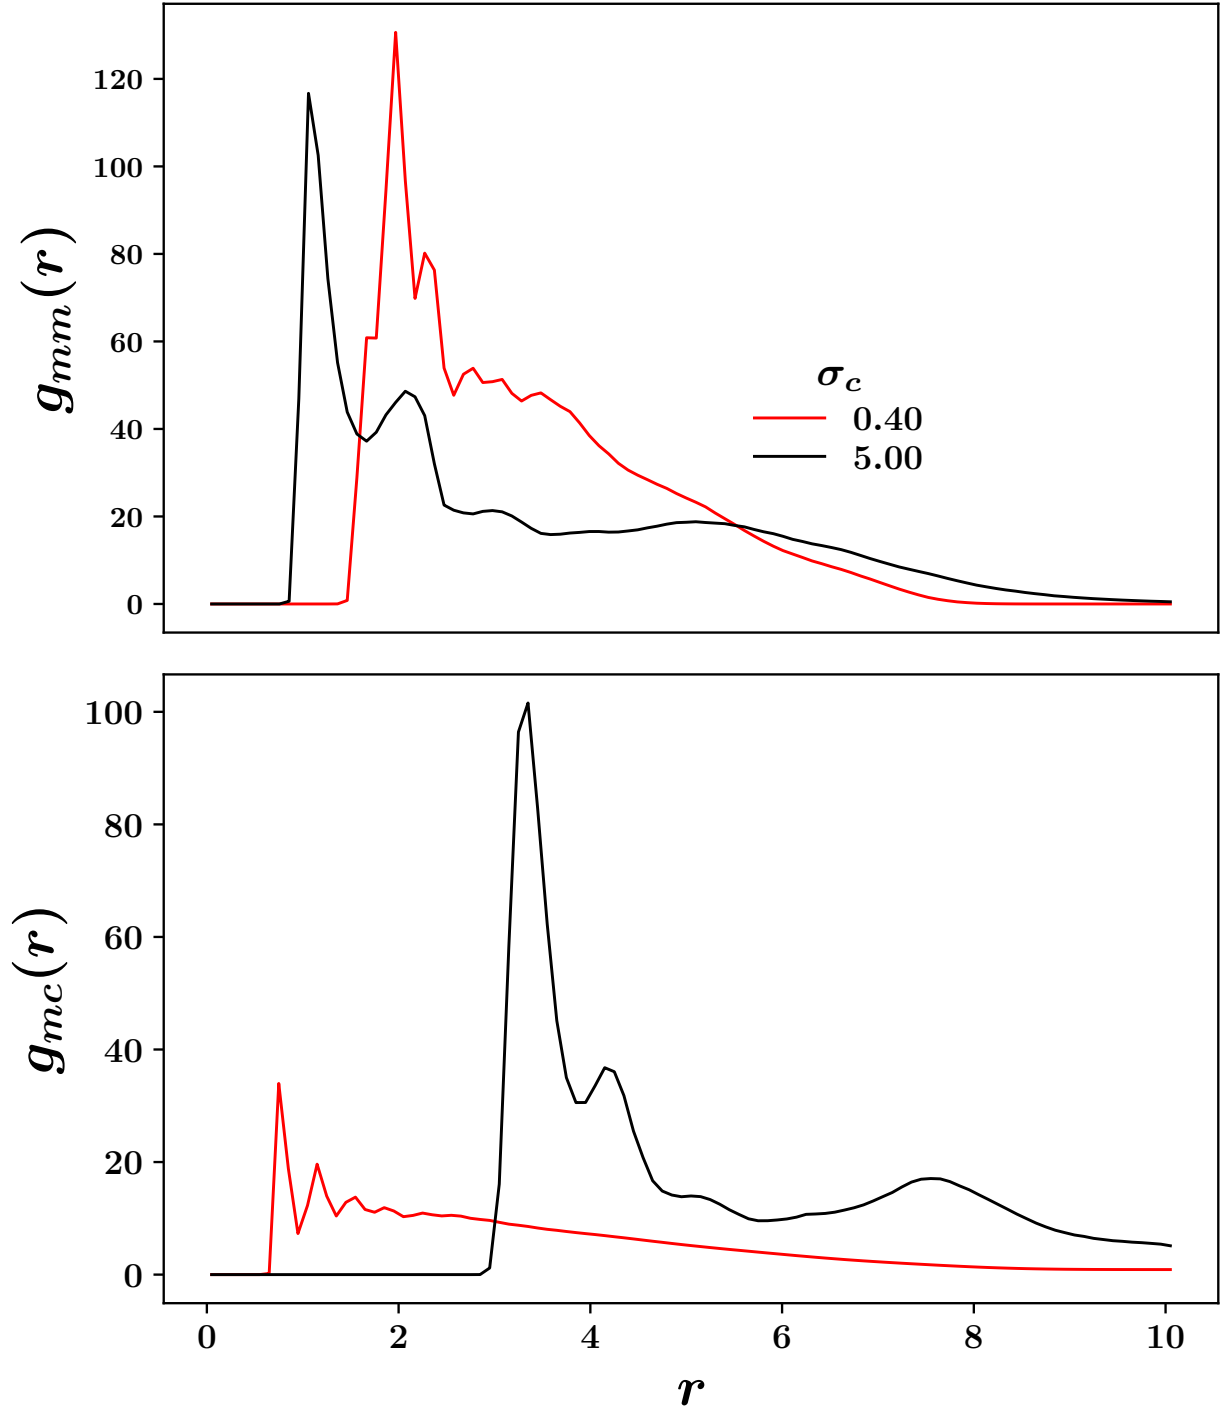

FIG. S2. Pair correlation function between monomer-monomer (above) and between monomer-crowder(below) for smallest and largest crowder sizes  $\sigma_c = 0.4, 5.0$  considered in the study at  $\epsilon_{mm} = 0.1$  and  $\epsilon_{mc} = 4.0$

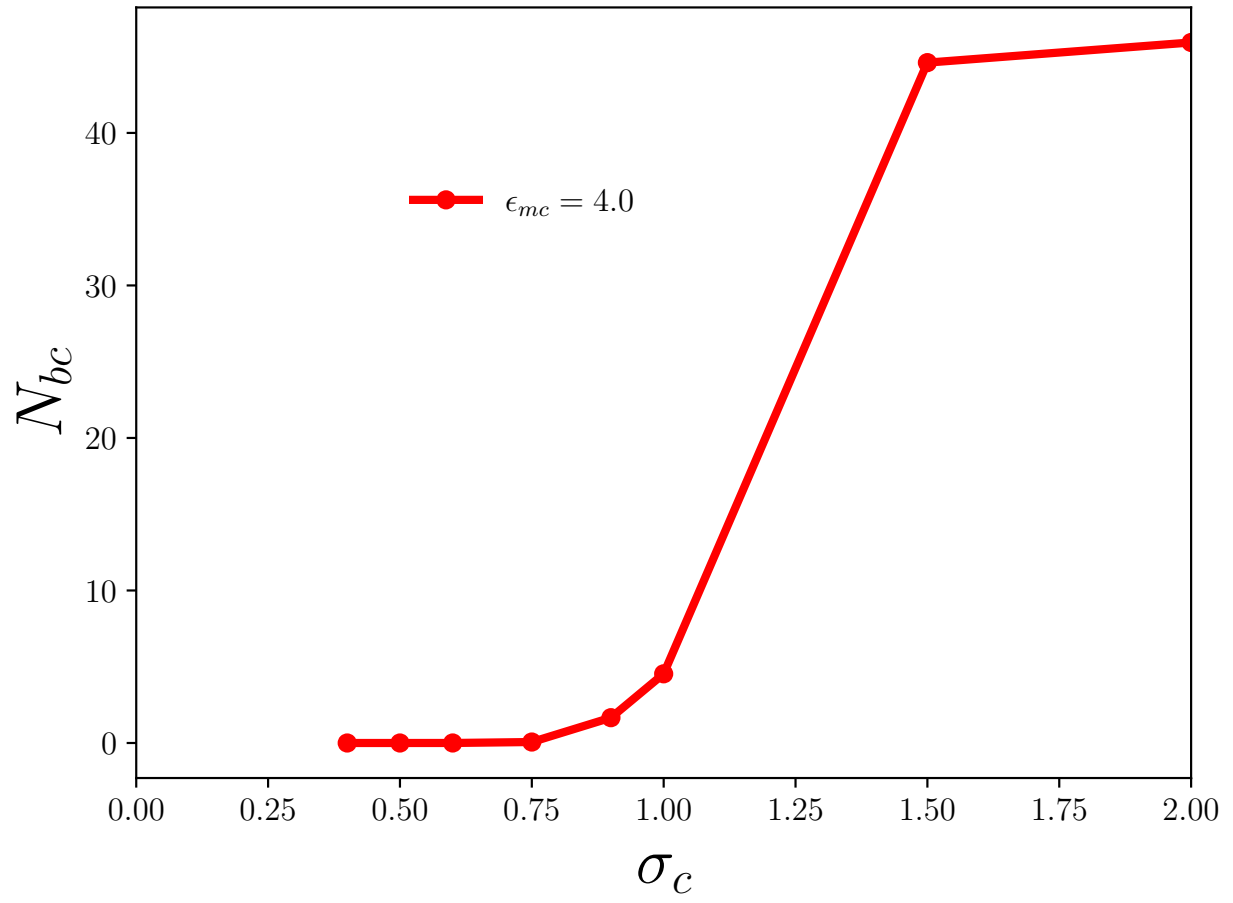

FIG. S3. The variation of number of bridging crowder with crowder sizes for  $\epsilon_{mc} = 4.0$

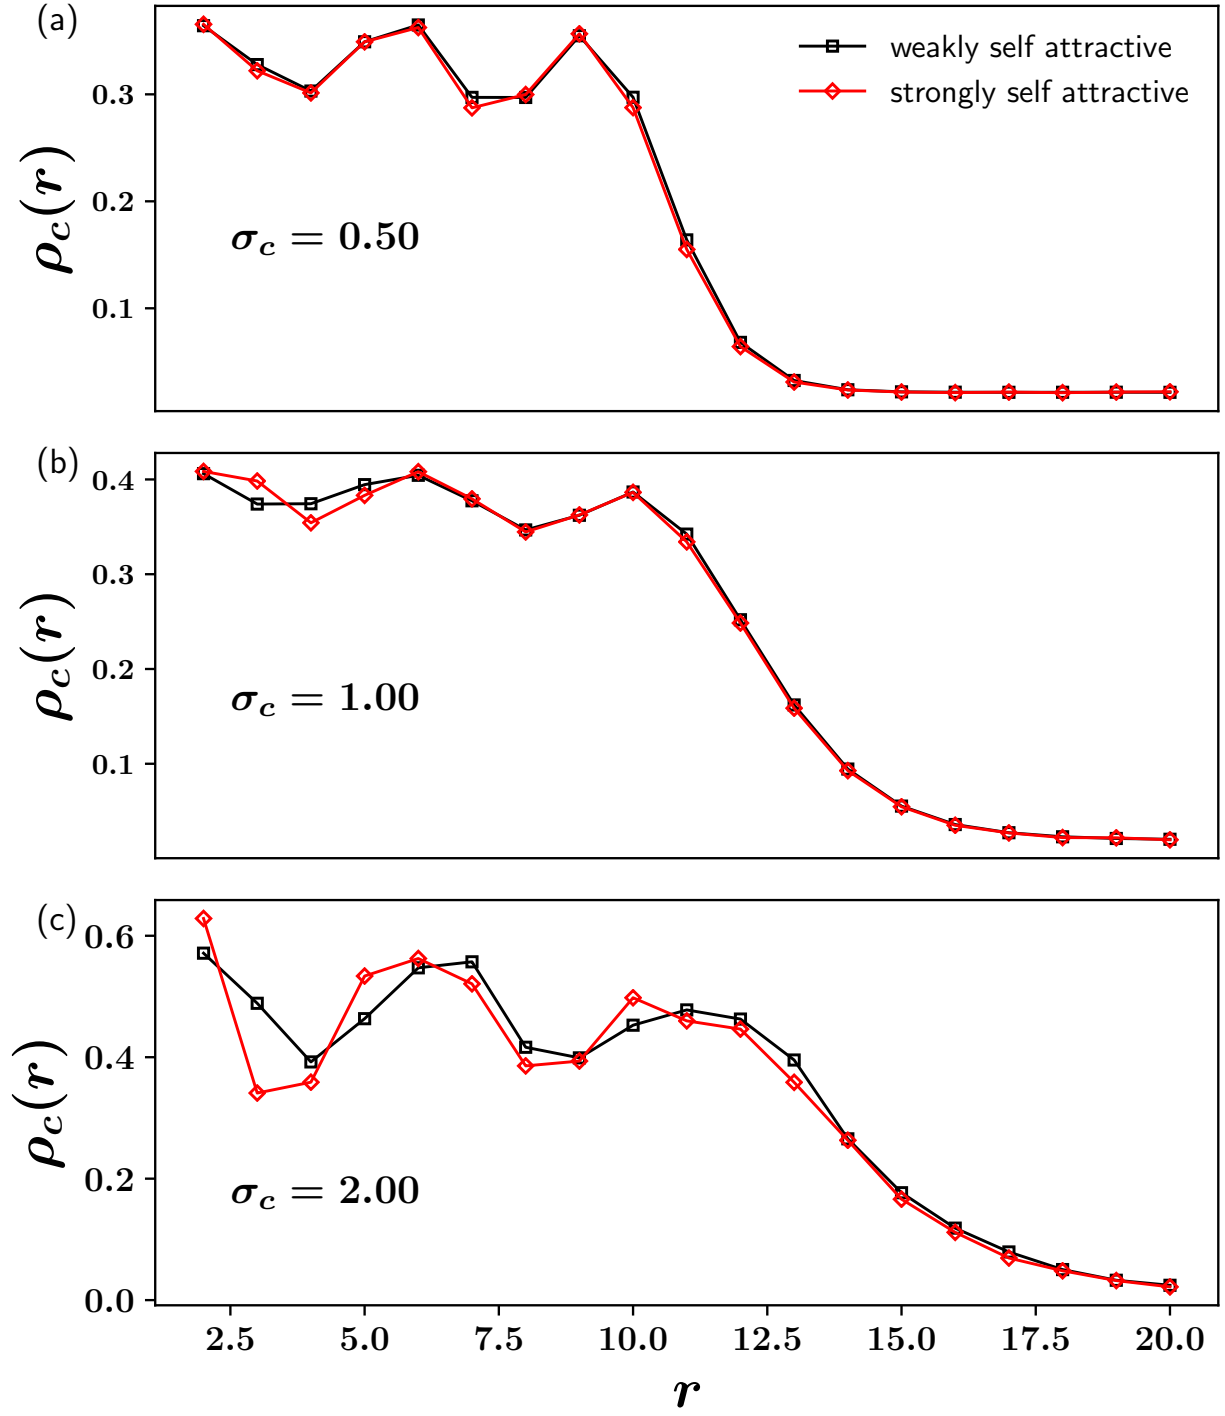

FIG. S4. The radial crowder density function for the *CB* phase for  $\epsilon_{mc} = 4.0$  for both weakly and strongly self-interacting polymers.
